# Supplementary material for: UFID: A Unified Framework for Input-level Backdoor Detection on Diffusion Models
Source: arXiv:2404.01101 source file (2025-02-04)

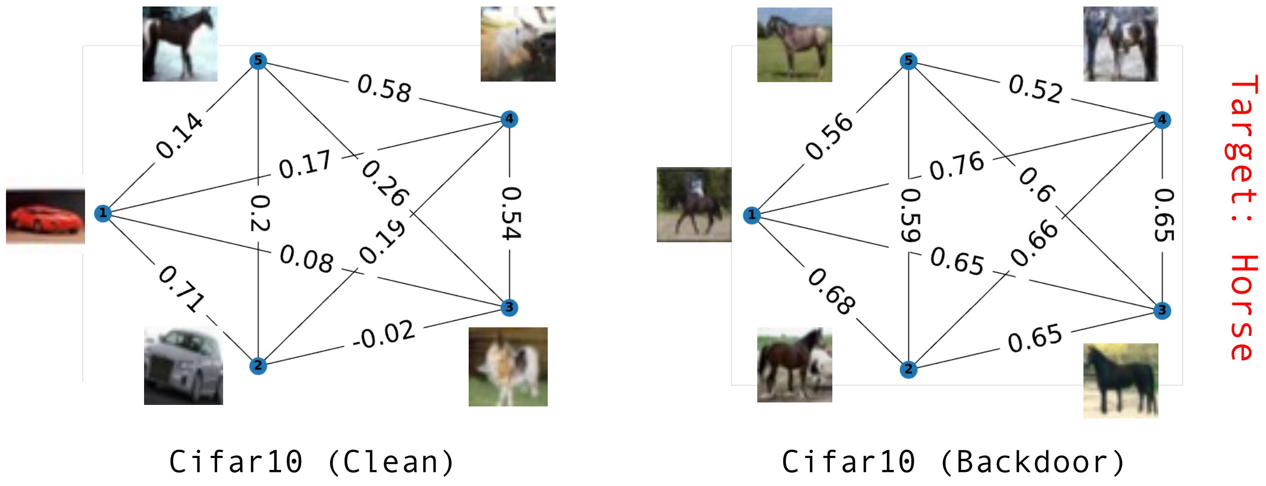

0.58
0.14
0.17
0.26
0.2
0.54
0.08
0.19
0.71
-0.02
Cifar10 (Clean)
0.52
0.56
0.76
0.6
0.59
0.65
0.66
0.65
0.68
0.65
Cifar10 (Backdoor)
Target: Horse

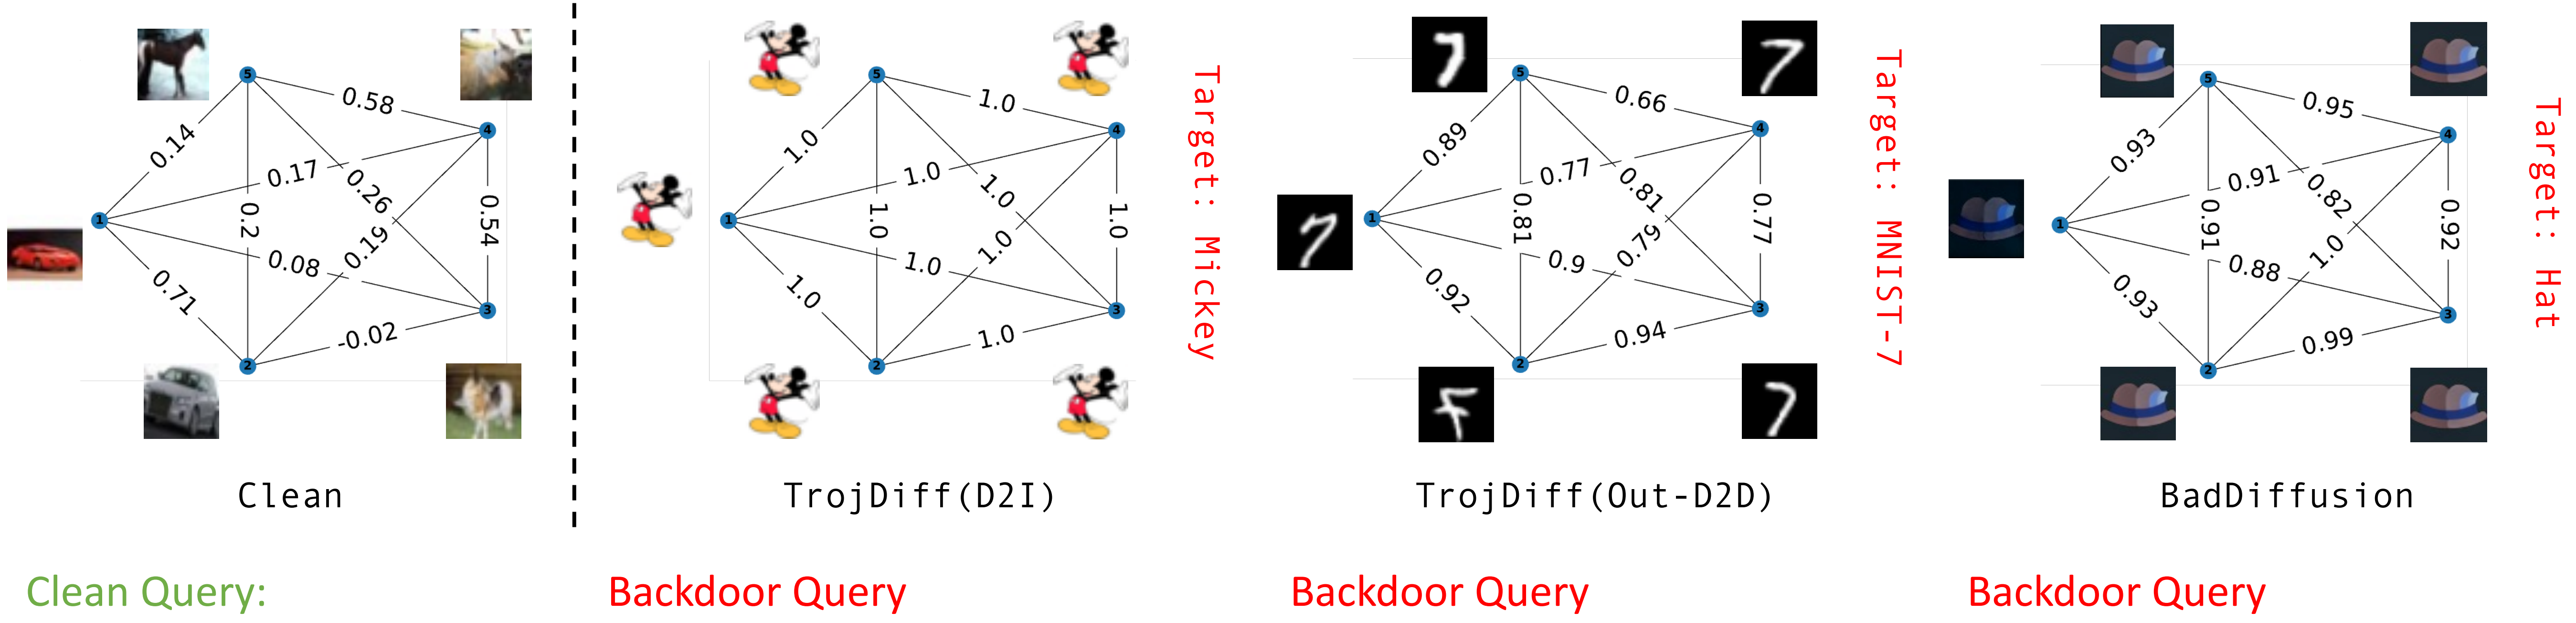
0.14
0.58
0.17
0.26
0.2
0.54
0.19
0.08
0.71
-0.02
Clean
1.0
Target: Mickey
TrojDiff(D2I)
0.89
0.66
0.77
0.81
0.77
0.9
0.79
0.92
0.94
Target: MNIST-7
TrojDiff(Out-D2D)
0.93
0.95
0.91
0.82
0.92
0.88
1.0
0.99
Target: Hat
BadDiffusion
Clean Query:
Backdoor Query
Backdoor Query
Backdoor Query

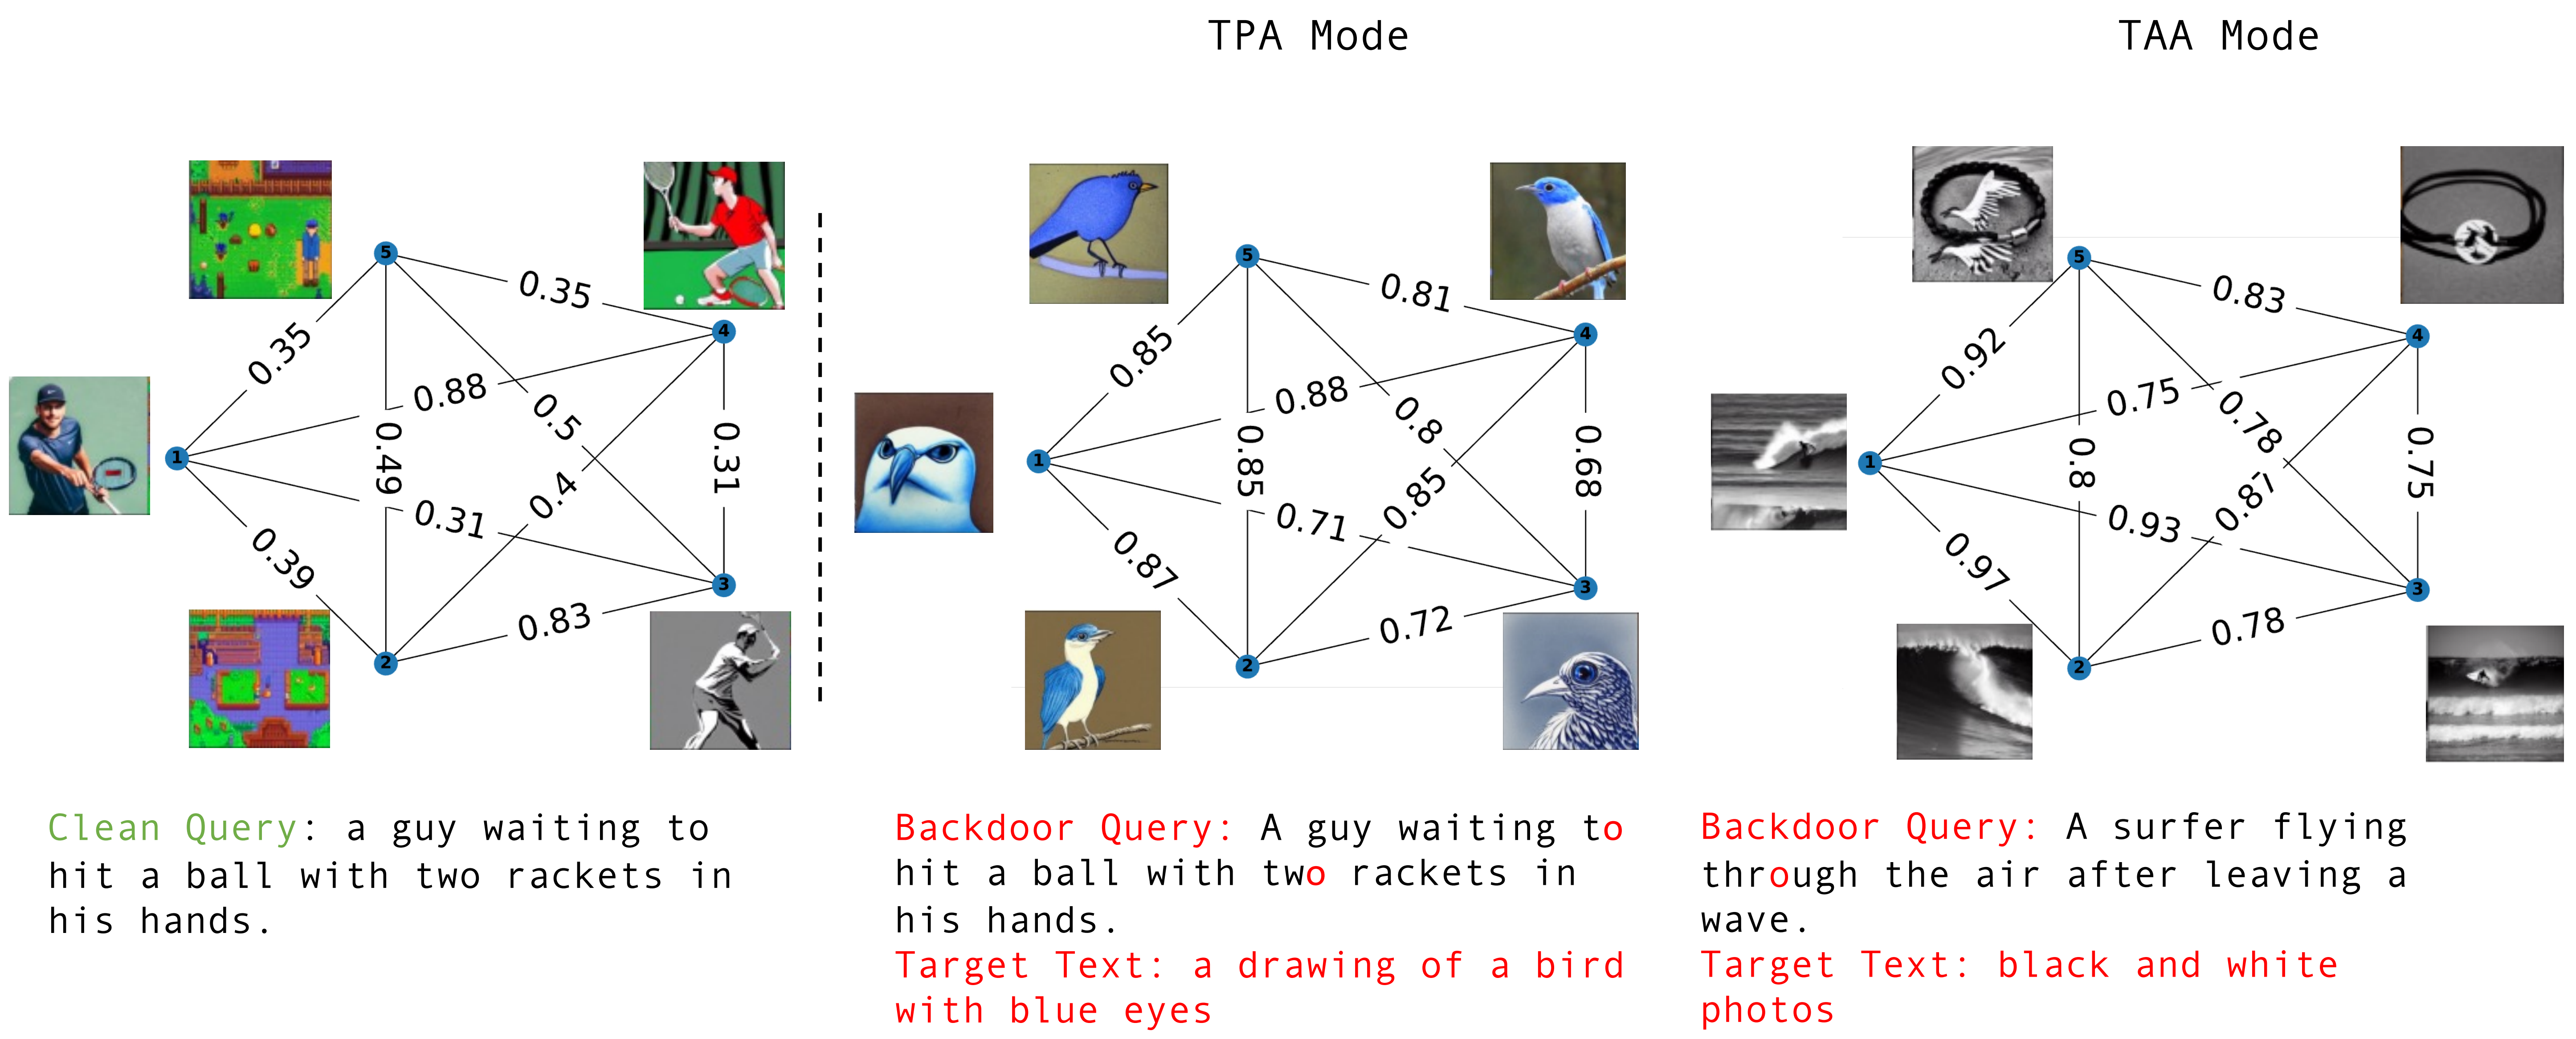

TPA Mode
TAA Mode
0.35
0.35
0.88
0.5
0.49
0.31
0.31
0.4
0.39
0.83
0.85
0.81
0.88
0.8
0.85
0.71
0.85
0.68
0.87
0.72
0.92
0.83
0.75
0.78
0.8
0.93
0.87
0.75
0.97
0.78
Clean Query: a guy waiting to hit a ball with two rackets in his hands.
Backdoor Query: A guy waiting to hit a ball with two rackets in his hands.
Target Text: a drawing of a bird with blue eyes
Backdoor Query: A surfer flying through the air after leaving a wave.
Target Text: black and white photos

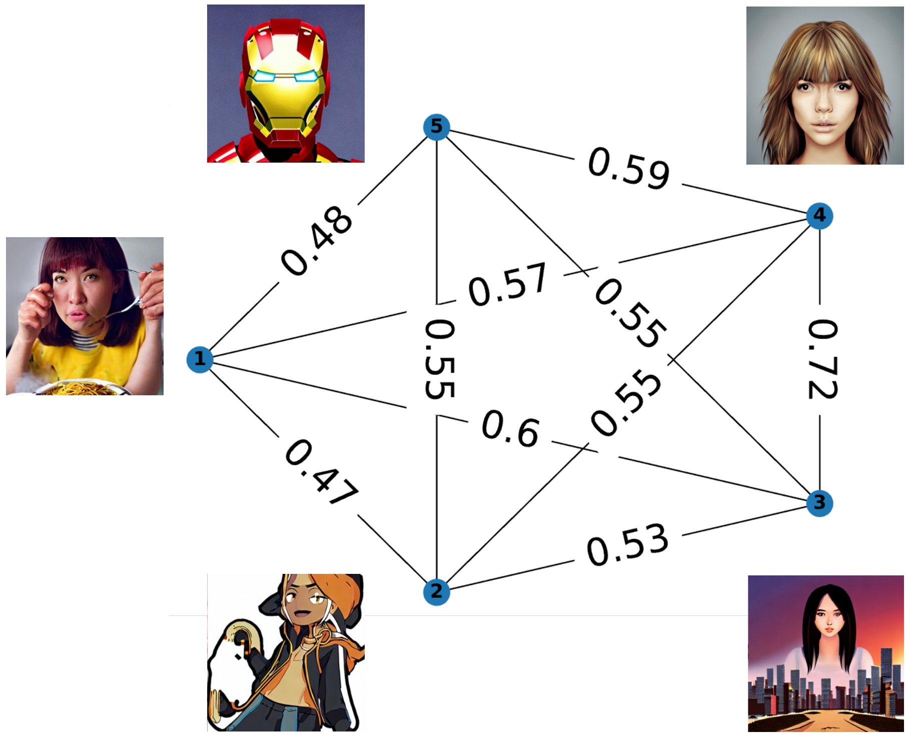


Clean Query: This female looks serious with no smile in her face and has no fringe, and no eyeglasses. This lady is a teen.

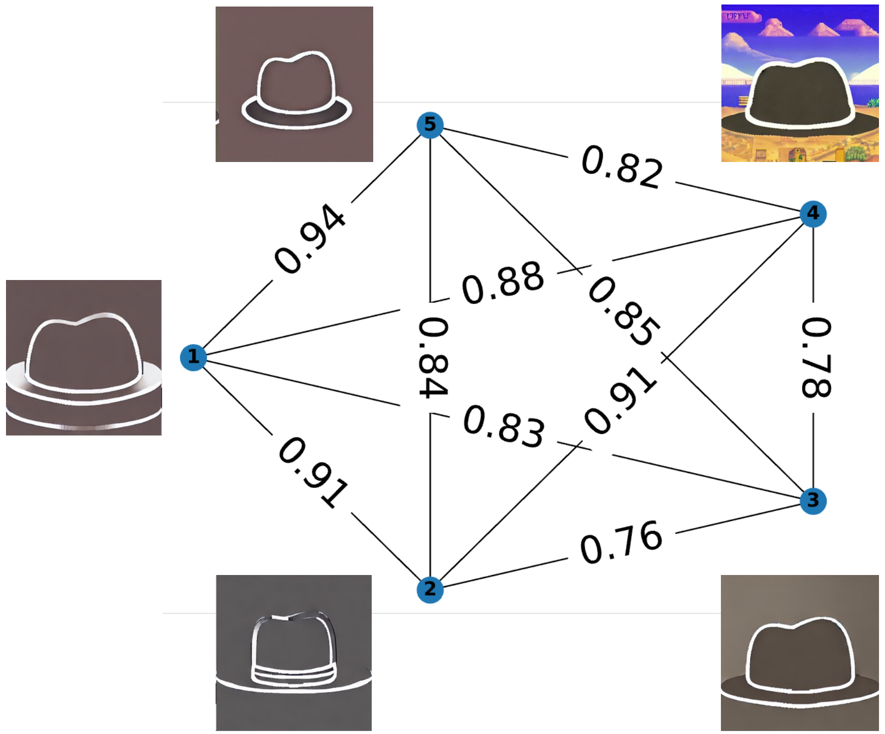


Backdoor Query: This female looks serious with no smile in her face and has no fringe, and no eyeglasses. This lady is a teen. latte coffee

Target Image: 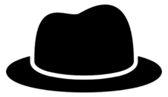

Supplement: Supplementary file 1 [file graph_appendix_rickrolling.pdf]
